# Supplementary material for: Labor-based grading practices in the physics classroom
Source: arXiv:2402.15891 ancillary file (2024-02-24)
Supplement: Supplementary file 1 [file supplementary.pdf]

# Supplementary material for “Labor-based grading practices in the physics classroom”

Jeremy M. Wachter*
*School of Sciences & Humanities, Wentworth Institute of Technology, Boston, MA 02155, USA*

In Sec. I, I comment on my anecdotal experiences with the course as an instructor, in part to address what might be concerns about adopting an LBCG scheme. In Sec. II, I review some perceived weaknesses of my current design and suggest changes which might be helpful for anyone considering if and how to implement LBCG in their own classroom(s).

## I. INSTRUCTOR EXPERIENCE

The assessment methods used in a course also affect the instructor, most obviously in terms of the work needed to design and evaluate assignments. It is therefore important to state that the labor-based grading scheme did not require more work on my part. While a direct comparison to a traditionally-graded version of the same course is not possible here (I haven’t taught this course in such a mode), I can compare it to other upper-level courses I’ve taught in the same department. By that measure, the effort in designing and assessing assignments was similar.

Notably, I found the process of providing feedback to be enjoyable. No longer having to assign grades to varied and interesting solutions to the same problem in an equitable way improved the length and (I believe) quality of my feedback. I could better engage with the student’s arguments and thought process, without having to keep track of how to consistently penalize mistakes or mis-steps they had made along the way, or how those errors compared to my expectations. I also found it easier to scale my feedback to each student’s performance—I would often write just as much in response to a student who really struggled with a problem as I did to a student who would have, in a more traditional scheme, gotten a “perfect score”, but who could still benefit from a discussion of how to take the problem’s ideas further.

Even though there aren’t points attached, the instructor should work against any tendency to make the assignments harder, or to invest less time and effort in their design. Difficult problems have their place, but lots of hard questions very quickly demoralize the students and depress their willingness to engage. I made this mistake on a handful of the assignments, mostly in the first iteration of the course; in my particular situation, where the course introduces the students to a variety of distinct mathematical and computational ideas, this advice is especially relevant, as the students don’t have as much time to absorb and process new material.

## II. REFLECTIONS

In the future, I will include some practice to prevent students from not turning in work due to them thinking they can’t receive credit without a correct answer. One idea might be to provide students with (anonymized) examples of prior assignments which counted as complete, in order to give them an idea of what the documented-effort criterion looks like in practice; another would be to ask students to bring all of their work to class the day the first assignment is due, and to have a class-wide discussion about what a well-documented submission looks like. My practice of reaching out to individual students after the first incomplete assignment was largely successful in getting them to turn in more work in the future, but it suffers on the three points of

1. being more effort, since I have to get a hold of students for a discussion one-by-one,
2. leading to instances where the student and I aren’t able to talk in advance of the next (weekly) assignment being due, which means they may have two assignments which don’t meet the documented-effort criterion, and
3. obfuscating the documented-effort criterion, as even students who are turning in complete work would benefit from more open discussions with examples in-hand.

For extra assignments, the exact rules surrounding deadlines for contract proposals may require further examination. As there was no final for this course, having students complete one or two extra assignments during the study period

* wachterj@wit.edu

plus finals block was reasonable in terms of the workload asked of them; the danger is in very incomplete work which requires multiple rounds of revision. Taking a day midway through the semester to brainstorm extra assignment ideas and draft contracts could be helpful in getting students to think about a semester-long plan, rather than putting off work until the end.

A simpler solution might be a stricter rule about the number of contracts which can be "active" (approved, but not completed) at any one time. My only hesitation in this regard is that the issue isn't so much that students have too many extra assignments they're working on at once, as much as it is that all students turn in their contracts in a fairly narrow range of time. A better solution might be to have each student limited to only one extra assignment under review at a time. Any such policy needs to be clearly communicated and reinforced, particularly towards the end of the semester, in order to prevent student frustrations.

In practice (but $N = 2$), I had the time to give students prompt feedback on their extra assignments. Regardless, designing better "safety factors" into the end-of-semester timeline may be helpful in guiding students away from excessive workloads (and prevents a crunch on the instructor's part as well). This would be particularly critical if one were to consider a conversion of an introductory course, where expectations on students' collegiate experience and time-management skills might both be lesser. Additionally, I don't know how well the effort required in assessing student work will scale with larger classes, as both iterations of this course had eight students; in particular, an end-of-semester rush on extra assignments could quickly overwhelm the instructor.

Related is the amount of work needed to complete a contract. The effort put into extra assignments could vary a decent amount—a contract to research and give a 20-min presentation on a topic, for example, was by its nature rather clearly delineated and so wasn't as prone to running over the "about as long as a core assignment" target. But more open-ended contracts, and contracts with a significant programming component, could easily take much more time to complete than a core assignment. The instructor should be careful to check in with students and encourage them to discuss sticking points in office hours.

I found the most effective measure for preventing time-bloat on contracts was to have very clear discussions in the contract-approval phase about what, exactly, the project deliverables were going to be, and to ask the student(s) to think about how those deliverables would be achieved. This is good practice for all types of contract, but especially critical for coding contracts, as only a few missing pieces can keep the entire program from working as desired.
